# Supplementary material for: Learning to Predict Trustworthiness with Steep Slope Loss
Source: arXiv:2110.00054 source file (2021-10-27)
Supplement: Supplementary file 1 [file suppl.tex]

\documentclass{article}

% if you need to pass options to natbib, use, e.g.:
%     \PassOptionsToPackage{numbers, compress}{natbib}
% before loading neurips_2021

% ready for submission
\usepackage[final]{neurips_2021}

% to compile a preprint version, e.g., for submission to arXiv, add add the
% [preprint] option:
%     \usepackage[preprint]{neurips_2021}

% to compile a camera-ready version, add the [final] option, e.g.:
%     \usepackage[final]{neurips_2021}

% to avoid loading the natbib package, add option nonatbib:
%    \usepackage[nonatbib]{neurips_2021}

\usepackage[utf8]{inputenc} % allow utf-8 input
\usepackage[T1]{fontenc}    % use 8-bit T1 fonts
\usepackage{hyperref}       % hyperlinks
\usepackage{url}            % simple URL typesetting
\usepackage{booktabs}       % professional-quality tables
\usepackage{amsfonts}       % blackboard math symbols
\usepackage{nicefrac}       % compact symbols for 1/2, etc.
\usepackage{microtype}      % microtypography
\usepackage{xcolor}         % colors

\usepackage{bm}
\usepackage{subfig}
\usepackage{capt-of}
\usepackage{mathtools}
\usepackage{siunitx}
\usepackage[figurename=Figure]{caption}
\usepackage{scrextend}
\usepackage{xspace}
\usepackage{xcolor}
\usepackage{multirow}
\usepackage{wrapfig}
\usepackage{amsmath}
\usepackage{amssymb}
\usepackage{amsthm}
\usepackage{thmtools}
% \usepackage{mathbbol}
%\usepackage{subcaption}
%\floatsetup[table]{capposition=top}
\usepackage{algorithm}      % algorithm
\usepackage[noend]{algpseudocode} % algorithm
\usepackage[title]{appendix}
\usepackage[export]{adjustbox}
\usepackage{fixltx2e}
\usepackage{booktabs}
\usepackage{textcomp}

\usepackage{xr}
\makeatletter
\newcommand*{\addFileDependency}[1]{% argument=file name and extension
	\typeout{(#1)}
	\@addtofilelist{#1}
	\IfFileExists{#1}{}{\typeout{No file #1.}}
}
\makeatother
\newcommand*{\myexternaldocument}[1]{%
	\externaldocument{#1}%
	\addFileDependency{#1.tex}%
	\addFileDependency{#1.aux}%
}
\myexternaldocument{main}

\newcounter{algsubstate}

% \newfloatcommand{capbtabbox}{table}[][\FBwidth]
% \floatsetup{heightadjust=object}

% Include other packages here, before hyperref.

% If you comment hyperref and then uncomment it, you should delete
% egpaper.aux before re-running latex.  (Or just hit 'q' on the first latex
% run, let it finish, and you should be clear).

\newtheorem*{theorem*}{Theorem}

% \newcommand{\eqref}[1]{\mbox{Equation~(\ref{#1})}}
% Have to use \renewcommand because exists already in amsmath
\renewcommand{\eqref}[1]{\mbox{Eq.~(\ref{#1})}}

\newcolumntype{L}[1]{>{\raggedright\arraybackslash}p{#1}}
\newcolumntype{C}[1]{>{\centering\arraybackslash}p{#1}}
\newcolumntype{R}[1]{>{\raggedleft\arraybackslash}p{#1}}

%\makeatletter
%\def\BState{\State\hskip-\ALG@thistlm}
%\makeatother
%%\floatname{algorithm}{Procedure}
%\renewcommand{\algorithmicrequire}{\textbf{Input:}}
%\renewcommand{\algorithmicensure}{\textbf{Output:}}
\makeatletter
% Reinsert missing \algbackskip
\def\algbackskip{\hskip-\ALG@thistlm}
\makeatother

\title{Appendix for Learning to Predict Trustworthiness with Steep Slope Loss}

% \author{%
%   Yan Luo \\
%   Dept. of Computer Science \& Engineering\\
%   University of Minnesota\\
%   \texttt{luoxx648@umn.edu} \\
%   \And  
%   Yongkang Wong \\
%   School of Computing \\
%   National University of Singapore \\
%   \texttt{yongkang.wong@nus.edu.sg} \\
%   \And  
%   Mohan S. Kankanhalli \\
%   School of Computing \\
%   National University of Singapore \\
%   \texttt{mohan@comp.nus.edu.sg} \\
%   \And
%   Qi Zhao \\
%   Dept. of Computer Science \& Engineering\\
%   University of Minnesota\\
%   \texttt{qzhao@cs.umn.edu} \\
% }
\author{
    Yan~Luo$^\dagger$, \ Yongkang~Wong$^\ddagger$, \ Mohan~S~Kankanhalli$^\ddagger$, \ Qi~Zhao$^\dagger$ \\
    \vspace{-2ex}\\
    $^\dagger$ Department of Computer Science \& Engineering, University of Minnesota\\
    $\ddagger$ School of Computing, National University of Singapore \\
    \vspace{-2ex}\\
    {\small \texttt{luoxx648@umn.edu}, \texttt{yongkang.wong@nus.edu.sg}, \texttt{mohan@comp.nus.edu.sg}, \texttt{qzhao@cs.umn.edu} }
}

\begin{document}

\maketitle

\input{sec/appendix}

\bibliographystyle{unsrt}
\bibliography{sec/references}

\end{document}
